# Supplementary material for: Short-Range Solvent-Solvent and Ion-Solvent Correlations at Metal-Electrolyte Interfaces: Parameterization and Benchmarking
Source: arXiv:2509.19213 ancillary file (2026-03-20)
Supplement: Supplementary file 1 [file Supporting_Materials.pdf]

# Supporting Materials for Short-Range Solvent–Solvent and Ion–Solvent Correlations at Metal–Electrolyte Interfaces: Parameterization and Benchmarking

Mengke Zhang<sup>\*</sup>

*Institute of Energy Technologies, IET-3: Theory and Computation of Energy Materials,  
Forschungszentrum Jülich GmbH, 52425 Jülich, Germany*

Jun Huang<sup>†</sup>

*Institute of Energy Technologies, IET-3: Theory and Computation of Energy Materials,  
Forschungszentrum Jülich GmbH, 52425 Jülich, Germany and*

*Theory of Electrocatalytic Interfaces,  
Faculty of Georesources and Materials Engineering,  
RWTH Aachen University, 52062 Aachen, Germany*

(Dated: September 11, 2025)

## CONTENTS

|                                                                                            |    |
|--------------------------------------------------------------------------------------------|----|
| I. Dielectric susceptibility of solvent orientational polarization                         | 2  |
| II. Nonlocal electrostatics                                                                | 3  |
| III. Smeared charge effect and short-range ion–solvent correlation effect on ion solvation | 5  |
| IV. Implementation of DPPFT model                                                          | 6  |
| V. Model parameters                                                                        | 9  |
| VI. Spatial distribution of infrared dielectric constant                                   | 10 |
| References                                                                                 | 10 |

---

<sup>\*</sup> [menkez@mail.ustc.edu.cn](mailto:menkez@mail.ustc.edu.cn)

<sup>†</sup> [ju.huang@fz.juelich.de](mailto:ju.huang@fz.juelich.de)

# I. DIELECTRIC SUSCEPTIBILITY OF SOLVENT ORIENTATIONAL POLARIZATION

The dielectric susceptibility distribution in real space corresponding to the spectrum in Eq. 5 can be obtained via the inverse Fourier transform as:

$$\begin{aligned}
\chi(r) &= \frac{1}{(2\pi)^3} \int d\mathbf{k} \chi(k) e^{i\mathbf{k} \cdot \mathbf{r}} \\
&= \frac{1}{(2\pi)^2} \int_0^\infty dk k^2 \chi(k) \int_0^\pi d\theta \sin \theta \cdot e^{ikr \cos \theta} \\
&= \frac{1}{(2\pi)^2} \int_0^\infty dk k^2 \chi(k) \cdot \frac{2 \sin(kr)}{kr} \\
&= \frac{1}{4\pi^2 r} \int_{-\infty}^{+\infty} dk \frac{k \sin(kr)}{\chi_0^{-1} + \varepsilon_{\text{ir}} K_\alpha k^2 + \varepsilon_{\text{ir}} K_\beta k^4} \\
&= \frac{1}{i8\pi^2 r} \int_{-\infty}^{+\infty} dk (f_+ - f_-), \tag{S1}
\end{aligned}$$

with

$$f_\pm = \frac{k \cdot e^{\pm ikr}}{\chi_0^{-1} + \varepsilon_{\text{ir}} K_\alpha k^2 + \varepsilon_{\text{ir}} K_\beta k^4}. \tag{S2}$$

By extending  $f_\pm$  to complex plane, provided that  $K_\alpha$  is negative and  $K_\beta$  is positive, the poles of the corresponding complex functions can be found either in the upper plane or the lower plane only if the below condition is satisfied:

$$(iX)^2 = K_\alpha^2 - 4K_\beta(\chi_0 \varepsilon_{\text{ir}})^{-1} = K_\alpha^2 - \gamma_0 K_\beta < 0, \tag{S3}$$

where  $X = (K_\beta \gamma_0 - K_\alpha^2)^{\frac{1}{2}} > 0$  with  $\gamma_0 = 4(\chi_0 \varepsilon_{\text{ir}})^{-1}$ . The poles can be solved from  $z^2 = (-K_\alpha \pm iX)/(2K_\beta)$  as:

$$z_1 = a + bi, \quad z_2 = a - bi, \quad z_3 = -a + bi, \quad z_4 = -a - bi, \tag{S4}$$

with

$$a = \sqrt{\frac{-K_\alpha + \sqrt{K_\alpha^2 + X^2}}{4K_\beta}} = \sqrt{\frac{-K_\alpha + \sqrt{K_\beta \gamma_0}}{4K_\beta}}, \tag{S5}$$

$$b = \sqrt{\frac{K_\alpha + \sqrt{K_\alpha^2 + X^2}}{4K_\beta}} = \sqrt{\frac{K_\alpha + \sqrt{K_\beta \gamma_0}}{4K_\beta}}. \tag{S6}$$

According to the residue theorem, dielectric susceptibility in Eq. S1 is calculated as

$$\begin{aligned}
\chi(r) &= \frac{1}{4\pi r} (Res\{f_+, z_1, +\} Res\{f_+, z_3, +\} Res\{f_-, z_2, +\} Res\{f_-, z_3, -\}) \\
&= \frac{1}{4\pi r} \left( \frac{e^{iz_1 r}}{2\varepsilon_{\text{ir}} K_\alpha + 4\varepsilon_{\text{ir}} K_\beta z_1^2} + \frac{e^{iz_3 r}}{2\varepsilon_{\text{ir}} K_\alpha + 4\varepsilon_{\text{ir}} K_\beta z_3^2} \right. \\
&\quad \left. + \frac{e^{-iz_2 r}}{2\varepsilon_{\text{ir}} K_\alpha + 4\varepsilon_{\text{ir}} K_\beta z_2^2} + \frac{e^{-iz_4 r}}{2\varepsilon_{\text{ir}} K_\alpha + 4\varepsilon_{\text{ir}} K_\beta z_4^2} \right) \\
&= \frac{1}{8\varepsilon_{\text{ir}} \pi r} \left( \frac{2e^{iz_1 r}}{K_\alpha + 2K_\beta z_1^2} + \frac{2e^{-iz_2 r}}{K_\alpha + 2K_\beta z_2^2} \right) \\
&= \frac{1}{4\varepsilon_{\text{ir}} \pi r} \frac{(K_\alpha + 2K_\beta z_1^2)e^{iar}e^{-br} + (K_\alpha + 2K_\beta z_2^2)e^{-iar}e^{-br}}{(K_\alpha + 2K_\beta z_1^2)(K_\alpha + 2K_\beta z_2^2)} \\
&= \frac{1}{4\varepsilon_{\text{ir}} \pi} \frac{2(K_\alpha + 2K_\beta(a^2 - b^2)) \cos(ar) + 8K_\beta ab \sin(ar)}{(K_\alpha + 2K_\beta(a^2 - b^2))^2 + 16K_\beta^2 a^2 b^2} \frac{e^{-br}}{r} \\
&= \frac{1}{4\varepsilon_{\text{ir}} \pi} \frac{8K_\beta ab \sin(ar)}{16K_\beta^2 a^2 b^2} \frac{e^{-br}}{r} \\
&= \frac{1}{4\varepsilon_{\text{ir}} \pi} \frac{1}{2K_\beta ab} \frac{\sin(ar)e^{-br}}{r} \\
&= \frac{\sin(ar)e^{-br}}{2\pi\varepsilon_{\text{ir}} X r}, \tag{S7}
\end{aligned}$$

with

$$a^2 - b^2 = \frac{-K_\alpha}{2K_\beta} = k_{\text{max}}^2, \quad ab = \frac{X}{4K_\beta}, \quad a^2 + b^2 = \sqrt{\frac{\gamma_0}{4K_\beta}}. \tag{S8}$$

Here,  $Res\{f_i, z_j, \}$  denotes the residue of the complex function  $f_i$  at its pole  $z_j$ . Inversely,  $K_\alpha$  and  $K_\beta$  can be expressed as functions of  $a$  and  $b$  as:

$$K_\alpha = -\frac{(a^2 - b^2)\gamma_0}{2(a^2 + b^2)^2}, \quad K_\beta = \frac{\gamma_0}{4(a^2 + b^2)^2}. \tag{S9}$$

## II. NONLOCAL ELECTROSTATICS

For an isotropic dielectric medium, the fundamental constitutive relation in electrostatics can be generalized to account for the nonlocal response, taking the form:

$$\mathbf{D}(\mathbf{r}) = \int d\mathbf{r}' \hat{\epsilon}(|\mathbf{r} - \mathbf{r}'|) \mathbf{E}(\mathbf{r}'). \tag{S10}$$

Here,  $\hat{\epsilon}$  denotes the nonlocal dielectric function, which is a scalar in an isotropic medium. Taking the gradient on both sides of the above equation yields

$$\nabla \cdot \mathbf{D} = - \sum_{\alpha, \beta=x,y,z} \frac{\partial}{\partial r_\alpha} \int d\mathbf{r}' \hat{\epsilon}(|\mathbf{r} - \mathbf{r}'|) \frac{\partial}{\partial r'_\beta} \phi(\mathbf{r}'). \tag{S11}$$

Here,  $r_\alpha$  and  $r_\beta$  denote the components of the position vector along the Cartesian coordinate axes  $\alpha$  and  $\beta$ , respectively. For a spherically symmetric charge density source,  $\rho(r)$ ,

Gauss's law in electrostatics provides

$$\nabla \cdot \mathbf{D} = - \sum_{\alpha, \beta=x,y,z} \frac{\partial}{\partial r_\alpha} \int d\mathbf{r}' \hat{\epsilon}(|\mathbf{r} - \mathbf{r}'|) \frac{\partial}{\partial r'_\beta} \phi(\mathbf{r}') = \rho(r), \quad (\text{S12})$$

Applying the Fourier transform to both sides of the above equation yields

$$\sum_{\alpha, \beta} k_\alpha k_\beta \hat{\epsilon}(k) \phi(k) = k^2 \epsilon(k) \phi(k) = \rho(k), \quad (\text{S13})$$

with

$$\phi(k) = \int d\mathbf{r} \phi(r) e^{-i\mathbf{k} \cdot \mathbf{r}}, \quad \hat{\epsilon}(k) = \int d\mathbf{r} \hat{\epsilon}(r) e^{-i\mathbf{k} \cdot \mathbf{r}}, \quad \rho(k) = \int d\mathbf{r} \rho(r) e^{-i\mathbf{k} \cdot \mathbf{r}}. \quad (\text{S14})$$

Here,  $\epsilon(k) = \sum_{\alpha, \beta} (k_\alpha k_\beta / k^2) \hat{\epsilon}(k)$  represents the longitudinal dielectric permittivity in Fourier space. According to Eq. S13, the electrostatic potential in Fourier space is expressed as

$$\phi(k) = \frac{\rho(k)}{k^2 \epsilon(k)}. \quad (\text{S15})$$

The ion solvation energy is then calculated as

$$\begin{aligned} \Delta G_{\text{solv}} &= \frac{1}{2} \int d\mathbf{r} \rho(r) [\phi(r) - \phi_{\text{vac}}(r)] \\ &= \frac{1}{2(2\pi^3)} \int d\mathbf{k} \rho(k) [\phi(k) - \phi_{\text{vac}}(k)] \\ &= \frac{1}{4\pi^2 \epsilon_0} \int_0^\infty dk \rho^2(k) \left( \frac{1}{\epsilon(k)} - 1 \right) \\ &= -\frac{1}{4\pi^2 \epsilon_0} \int_0^\infty dk \rho^2(k) \chi_{\text{tot}}(k), \end{aligned} \quad (\text{S16})$$

where  $\epsilon(k) = \epsilon(k)/\epsilon_0$ .

### III. SMEARED CHARGE EFFECT AND SHORT-RANGE ION-SOLVENT CORRELATION EFFECT ON ION SOLVATION

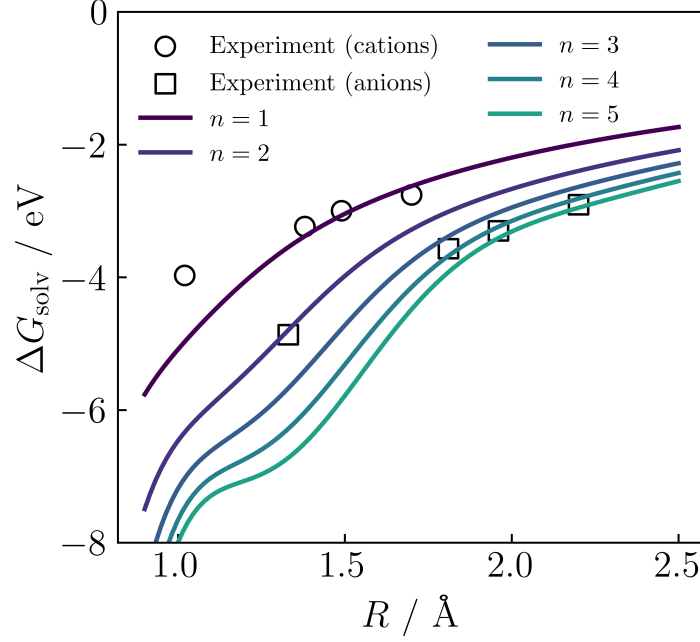

FIG. S1. Comparisons of experimental hydration energies of alkali metal cations (circles) and halide anions (squares) with those calculated from Eq. 19 using SGn model for the ionic charge distribution.  $n$  varies from 1 to 5, as indicated in the figure, while the short-range ion-solvent correlation parameter  $\alpha$  is set to zero in all model cases. Other parameters used are:  $K_\alpha = -0.047 \text{ \AA}^2$  (determined from Eq. 8),  $K_\beta = 0.0026 \text{ \AA}^4$  (determined from Eq. 8),  $\varepsilon_{\text{ir}} = 4.9$  (Ref. [1]),  $\varepsilon_s = 78.5$  (Ref. [1]). Ionic crystal radii are used for  $R$ , and their values together with the corresponding hydration energies are taken from Ref. [2].

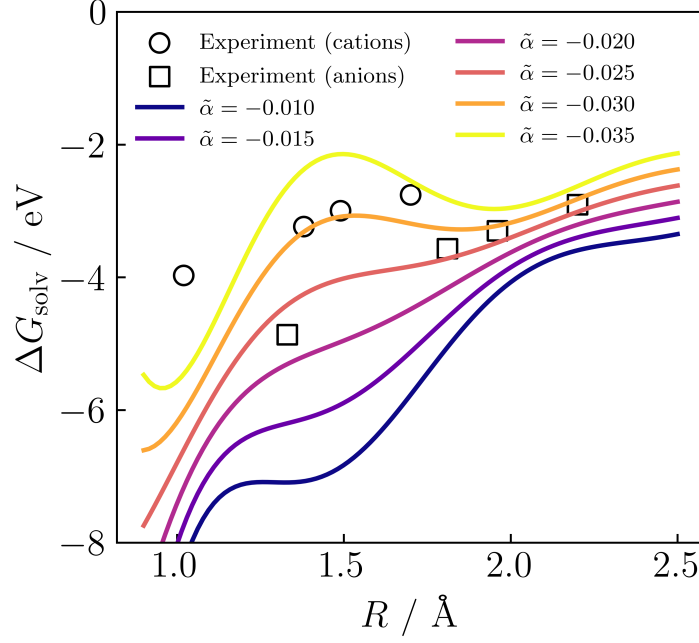

FIG. S2. Comparisons of experimental hydration energies of alkali metal cations (circles) and halide anions (squares) with those calculated from Eq. 19 using SGn model for the ionic charge distribution. The dimensionless short-range ion-solvent correlation parameter,  $\tilde{\alpha} = \alpha\epsilon_0/a_0^2$ , varies from  $-0.01$  to  $-0.035$ , as indicated in the figure, while the parameter  $n$  in the SGn model is set to 50 in all model cases.  $a_0 = 1$  Å is the referenced distance. Other parameters used are:  $K_\alpha = -0.047$  Å<sup>2</sup> (determined from Eq. 8),  $K_\beta = 0.0026$  Å<sup>4</sup> (determined from Eq. 8),  $\epsilon_{\text{ir}} = 4.9$  (Ref. [1]),  $\epsilon_s = 78.5$  (Ref. [1]). Ionic crystal radii are used for  $R$ , and their values together with the corresponding hydration energies are taken from Ref. [2].

#### IV. IMPLEMENTATION OF DPPFT MODEL

A detailed derivation of the DPPFT can be found in our previous work[3]. Within DPPFT, the kinetic and exchange-correlation energies of free electrons in the metal are described by the Thomas-Fermi-von Weizsäcker (TFvW) and Perdew-Burke-Ernzerhof (PBE) theories, respectively. The controlling equation for the electron density  $n_e$  is derived as

$$\begin{aligned} \tilde{\nabla}^2 \tilde{n}_e = & \frac{20}{3} \tilde{n}_e \frac{\omega}{\theta_{\text{T}}\omega - \theta_{\text{XC}}} \left( \frac{\partial t_{\text{TF}}}{\partial \tilde{n}_e} + \frac{\partial u_{\text{X}}^0}{\partial \tilde{n}_e} + \frac{\partial u_{\text{C}}^0}{\partial \tilde{n}_e} - \frac{\tilde{\mu}_e + e_0\phi}{e_{\text{au}}} \right) \\ & + \frac{\theta_{\text{T}}\omega - \frac{4}{3}\theta_{\text{XC}}}{2\tilde{n}_e(\theta_{\text{T}}\omega - \theta_{\text{XC}})} (\tilde{\nabla} \tilde{n}_e)^2, \end{aligned} \quad (\text{S17})$$

with,

$$t_{\text{TF}} = \frac{3}{10}(3\pi^2)^{\frac{2}{3}}(\tilde{n}_e)^{\frac{5}{3}}, \quad (\text{S18})$$

$$u_{\text{X}}^0 = -\frac{3}{4}\left(\frac{3}{\pi}\right)^{\frac{1}{3}}(\tilde{n}_e)^{\frac{4}{3}}, \quad (\text{S19})$$

$$u_{\text{C}}^0 = -2a_1(1 + a_2r_s)\tilde{n}_e \ln\left(\frac{1}{\xi} + 1\right), \quad (\text{S20})$$

$$\xi = 2a_1\left(a_3r_s^{\frac{1}{2}} + a_4r_s + a_5r_s^{\frac{3}{2}} + a_6r_s^2\right), \quad (\text{S21})$$

where the dimensionless electron density  $\tilde{n}_e = n_e a_0^3$ , the dimensionless gradient operator  $\tilde{\nabla} = a_0 \nabla$ , the radius  $r_s = \left(\frac{3}{4\pi\tilde{n}_e}\right)^{\frac{1}{3}}$ , the variable  $\omega = \frac{2}{5}(3\pi^5\tilde{n}_e)^{\frac{1}{3}}$ , the constant  $\theta_{\text{XC}} = \theta_{\text{X}} - \frac{\pi^2}{3}\theta_{\text{C}}$ , the atomic energy  $e_{\text{au}} = \frac{e_0^2}{4\pi\epsilon_0 a_0}$ .  $\tilde{\mu}_e$  is the electrochemical potential of electrons.  $\theta_{\text{T}}, \theta_{\text{X}}, \theta_{\text{C}}$  are coefficients tuning the contribution of the gradient term in the kinetic energy, the exchange energy, and the correlation energy of electrons, respectively.  $a_0, e_0, \epsilon_0$  are the Bohr radius, the elementary charge, the vacuum permittivity, respectively. The coefficients  $a_1 = 0.0310907, a_2 = 0.2137, a_3 = 7.5957, a_4 = 3.5876, a_5 = 1.6382, a_6 = 0.49294$ [4].

In one-dimensional case with the variable  $x$  representing the coordinate, the controlling equation for the electrostatic potential  $\phi$  is derived as,

$$\nabla(\epsilon_{\text{ir}}\nabla\phi - P) = -(n_{\text{c}} - n_{\text{a}} + n_{\text{cc}} - n_{\text{e}})e_0, \quad (\text{S22})$$

where  $n_{\text{c}}, n_{\text{a}}, n_{\text{cc}}$  are cation number density, anion number density, and the background charge density contributed by metal cationic cores, respectively. The positive direction of the polarization field is conventionally defined from the negative to the positive charge center, in contrast to the definition adopted in the previous work[3, 5–7].

The number density of electrolyte component  $i$  ( $i = a, c, s$ ) in a lattice model is expressed as,

$$n_i = n_{\text{max}} \frac{\chi_i \Theta_i}{\chi_v + \sum_i \gamma_i \chi_i \Theta_i}, \quad (\text{S23})$$

with the thermodynamic factor  $\Theta_i$  being,

$$\Theta_{\text{c}} = \exp(-\beta e_0(\phi - \alpha_{\text{c}}\nabla P) - \beta w_{\text{c}}), \quad (\text{S24})$$

$$\Theta_{\text{a}} = \exp(\beta e_0(\phi - \alpha_{\text{a}}\nabla P) - \beta w_{\text{a}}), \quad (\text{S25})$$

$$\Theta_{\text{s}} = \frac{\sinh(\beta p |\mathcal{E} + \nabla\phi|)}{\beta p |\mathcal{E} + \nabla\phi|} \exp(-\beta w_{\text{s}}), \quad (\text{S26})$$

where  $\chi_i = \frac{n_i^{\text{b}}}{n_{\text{max}}}$ ,  $n_i^{\text{b}}$  is the bulk number density of electrolyte component  $i$ .  $\Lambda_{\text{B}}$  and  $n_{\text{max}} = \Lambda_{\text{B}}^{-3} = (\sum_i n_i^{\text{b}} \gamma_i) / (1 - \chi_v)$  are the characteristic length and the maximum number density of referenced lattices, respectively.  $\gamma_i = (2r_i/\Lambda_{\text{B}})^3$ , where  $r_i$  is the radius of electrolyte component  $i$ .  $\chi_v$  is the fraction of vacancy lattices in bulk solution, *i.e.*,  $\chi_v = 1 - \sum_i \gamma_i \chi_i$ .

We use the repelling part of the Morse potential  $w_i$  for preventing electrolyte component  $i$  from penetrating into the metal phase. It's expressed as,

$$w_i = D_i \exp(-2\beta_i(d - d_i)) = k_{\text{B}}T \exp(-2\beta_i(d - d_i^{\text{M}})), \quad (\text{S27})$$

with the effective equilibrium distance of solution component  $i$  from the metal surface,

$$d_i^{\text{M}} = d_i + \frac{\ln(D_i/k_B T)}{2\beta_i}, \quad (\text{S28})$$

where  $D_i$  is the depth of the potential well,  $\beta_i$  is the coefficient controlling the width of potential well, and  $d, d_i$  are respectively the distance and the equilibrium distance from the positions of electrolyte particle  $i$  to the metal surface.

Eqs. S17, S22, 1 and 2 are solved as a set of coupled ordinary differential equations (ODEs) in COMSOL 6.1. The detailed settings for the COMSOL solver are provided in the Supplementary Materials of Ref. [3].



## V. MODEL PARAMETERS

TABLE S1. DPPFT model parameters at the Ag(111)–100 mM NaF aqueous solution interface.

| Symbol                      | Item                                                  | Value                    | Source                                                                         |
|-----------------------------|-------------------------------------------------------|--------------------------|--------------------------------------------------------------------------------|
| $a_1$                       | Coefficient in the PBE functional                     | 0.0310907                | Ref. [4]                                                                       |
| $a_2$                       | Coefficient in the PBE functional                     | 0.2137                   | Ref. [4]                                                                       |
| $a_3$                       | Coefficient in the PBE functional                     | 7.5957                   | Ref. [4]                                                                       |
| $a_4$                       | Coefficient in the PBE functional                     | 3.5876                   | Ref. [4]                                                                       |
| $a_5$                       | Coefficient in the PBE functional                     | 1.6382                   | Ref. [4]                                                                       |
| $a_6$                       | Coefficient in the PBE functional                     | 0.49294                  | Ref. [4]                                                                       |
| $\theta_X$                  | Gradient coefficient in the exchange functional       | 0.1235                   | Ref. [4]                                                                       |
| $\theta_C$                  | Gradient coefficient in the correlation functional    | 0.0667                   | Ref. [4]                                                                       |
| $\theta_T$                  | Gradient coefficient in the kinetic energy functional | 0.585                    | Fitted to experimental PZC at Ag(111)–100 mM NaF aqueous solution interface[8] |
| $\varepsilon_{\text{ir,M}}$ | Infrared dielectric constant of the metal             | 3                        | Ref. [9]                                                                       |
| $n_{cc}^0$                  | Charge density of metal cationic cores                | $0.645 \text{ \AA}^{-3}$ | 11 electrons per Ag atom                                                       |
| $c_s^b$                     | Bulk solvent concentration                            | $55600 \text{ mol/m}^3$  | Ref. [3]                                                                       |
| $r_c$                       | Radius of cations                                     | $1.02 \text{ \AA}$       | Ref. [2]                                                                       |
| $r_a$                       | Radius of anions                                      | $1.33 \text{ \AA}$       | Ref. [2]                                                                       |
| $\Lambda_B$                 | Diameter of solvent molecules                         | $2.75 \text{ \AA}$       | Ref. [10]                                                                      |
| $\varepsilon_{\text{ir,S}}$ | Infrared dielectric constant of the solution          | 4.9                      | Ref. [1]                                                                       |
| $\varepsilon_s$             | Static dielectric constant in the bulk solution       | 78.5                     | Ref. [11]                                                                      |
| $K_\alpha$                  | Short-range solvent–solvent correlation parameter     | $-0.0354 \text{ \AA}^2$  | Eq. 22                                                                         |
| $K_\beta$                   | Short-range solvent–solvent correlation parameter     | $0.00147 \text{ \AA}^4$  | Eq. 22                                                                         |
| $\alpha_c$                  | Short-range cation–solvent correlation parameter      | $-0.03 a_0^2/\epsilon_0$ | Eq. 19                                                                         |
| $\alpha_a$                  | Short-range anion–solvent correlation parameter       | $-0.02 a_0^2/\epsilon_0$ | Eq. 19                                                                         |
| $d_s^M$                     | Effective equilibrium distance of solvent molecules   | $2.1 \text{ \AA}$        | Ref. [12]                                                                      |
| $d_c^M$                     | Effective equilibrium distance of cations             | $3.2 \text{ \AA}$        | Ref. [12]                                                                      |
| $d_a^M$                     | Effective equilibrium distance of anions              | $4.2 \text{ \AA}$        | Ref. [12]                                                                      |

The effective equilibrium distances of  $\text{F}^-$ ,  $\text{Na}^+$ , and water molecules are chosen such that their closest approach to the metal surface is consistent with AIMD simulations[12].

## VI. SPATIAL DISTRIBUTION OF INFRARED DIELECTRIC CONSTANT

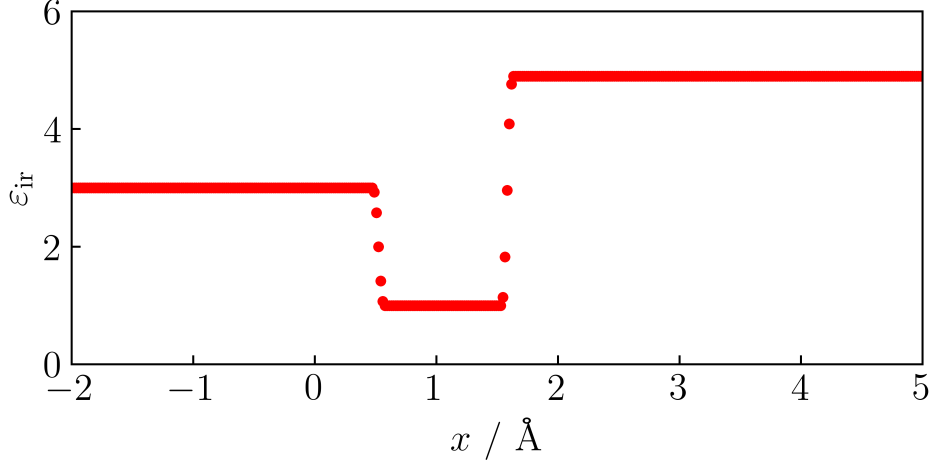

FIG. S3. Spatial distribution of the infrared dielectric constant in the DPPFT model. A vacuum region is present between the metal surface and the first water layer; the infrared dielectric constant is  $\epsilon_{\text{ir},\text{M}}$  to the left of this region (metal side) and  $\epsilon_{\text{ir},\text{S}}$  to the right (solution side).

- 
- [1] A. A. Kornyshev and G. Sutmann, *The Journal of chemical physics* **104**, 1524 (1996).
  - [2] Y. Marcus, *Ions in Solution and their Solvation* (John Wiley & Sons, 2015).
  - [3] M. Zhang, Y. Chen, M. Eikerling, and J. Huang, *Physical Review Applied* **23**, 024009 (2025).
  - [4] C. Fiolhais, F. Nogueira, and M. A. Marques, *A primer in density functional theory*, Vol. 620 (Springer, 2008).
  - [5] R. Blossey and R. Podgornik, *Physical Review Research* **4**, 023033 (2022).
  - [6] R. Blossey and R. Podgornik, *Journal of Physics A: Mathematical and Theoretical* **56**, 025002 (2023).
  - [7] R. Blossey and R. Podgornik, *Europhysics Letters* **139**, 27002 (2022).
  - [8] G. Valette, *Journal of electroanalytical chemistry and interfacial electrochemistry* **269**, 191 (1989).
  - [9] P. B. Johnson and R.-W. Christy, *Physical review B* **6**, 4370 (1972).
  - [10] K. Amann-Winkel, M.-C. Bellissent-Funel, L. E. Bove, T. Loerting, A. Nilsson, A. Pacia-roni, D. Schlesinger, and L. Skinner, *Chemical reviews* **116**, 7570 (2016).
  - [11] A. M. Kuznetsov and J. Ulstrup, *Electron transfer in chemistry and biology: an introduction to the theory* (John Wiley & Sons Ltd, 1999).
  - [12] L. Li, Y.-P. Liu, J.-B. Le, and J. Cheng, *Cell Reports Physical Science* **3** (2022).
